# Supplementary material for: One- and two-particle properties of the weakly interacting two-dimensional Hubbard model in proximity to the van Hove singularity
Source: arXiv:2203.09657 source file (2022-03-17)
Supplement: Supplementary file 1 [file charge_PRB_supplemental.pdf]

# Supplementary material for: One- and two-particle properties of the weakly interacting two-dimensional Hubbard model in proximity to the van Hove singularity


B. D. E. McNiven,[1] Hanna Terletska,[2] G. T. Andrews,[1] and J. P. F. LeBlanc[1,*]

[1]*Department of Physics and Physical Oceanography, Memorial University of Newfoundland, St. John's, Newfoundland & Labrador, Canada A1B 3X7*

[2]*Department of Physics and Astronomy, Computational Sciences Program, Middle Tennessee State University, Murfreesboro, TN 37132, USA*


| Expansion | $N^{(0)}$ | $N^{(1)}$ | $N^{(2)}$ | $N^{(3)}$ | $N^{(4)}$ | $N^{\text{terms}}$ |
|---|---|---|---|---|---|---|
| $\chi_{\uparrow\uparrow}$ | 1 | 0 | 4 | 14 | 93 | 23,327 |
| $\chi_{\uparrow\downarrow}$ | 0 | 1 | 2 | 13 | 78 | 17,954 |
| $D$ | 0 | 1 | 2 | 13 | 78 | 52,644 |

TABLE I. Number of diagrams for the Hubbard interaction at order $m$, $N^{(m)}$ for each expansion, and total number of analytic terms after processing with AMI, $N^{\text{terms}}$.

## I. SUPPLEMENTARY NOTE 1: DIAGRAMMATIC EXPANSIONS

We enumerate the number of diagrams at each order in the expansions of the susceptibilities $\chi_{\uparrow\uparrow}$ and $\chi_{\uparrow\downarrow}$ as well as the double occupancy $D$ in Table I. The diagrammatic expansions include those diagrams that are one-particle reducible in the bosonic channel. We sketch the first few diagrams in Figure S1.

The final column of Table I shows the total number of analytic terms generated by AMI up to 4th order. While the RPA approximation includes only a single diagram comprised of two analytic terms, the data we present for $\chi_s$ and $\chi_d$ includes 41,281 analytic terms. In the case of the double occupancy the diagrammatic expansion is identical to that of $\chi_{\uparrow\downarrow}$ but includes an additional summation over the external bosonic Matsubara frequency. This results in substantially more terms and somewhat higher computational expense per term.

In the case of results presented on the real frequency axis, we restrict calculations to third order. While this is substantially fewer diagrams it still represents 1604 analytic terms, far beyond anything previously accessible.

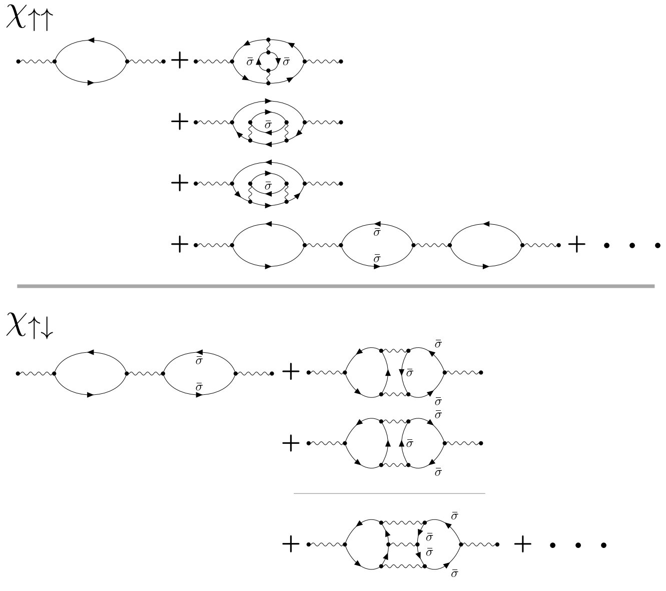


FIG. S1. First few diagrams in the expansions of $\chi_{\uparrow\uparrow}$ and $\chi_{\uparrow\downarrow}$. Due to the form of the Hubbard interaction, only interaction lines between propagators with opposite spins are non-zero. To track this, unmarked lines represent a spin choice $\sigma$ and marked lines have spin $\bar{\sigma}$ that is defined to be the opposite to $\sigma$.

## II. SUPPLEMENTARY NOTE 2: COMPARISONS TO NON-PERTURBATIVE METHODS

### A. Multi-peak Structure in Charge Susceptibility: DMFT+Dual Fermions

We compare the results of the static $\vec{q} = (\pi, \pi)$ spin and charge susceptibilities resulting from our many-body perturbation theory with algorithmic Matsubara integration (MBPT+AMI) technique to that of a non-perturbative method, DMFT+DF, displayed in Fig. S2.[1, 2] We perform the DF calculation for a finite momentum resolution of $64 \times 64$ points. The calculation involves the measurement of the 4-point vertex function within DMFT, $F^{\nu\nu'\omega}$, which we obtain on a truncated grid $\nu = \nu' = \{-64, ..., 64\}$ and $\omega = \{-24, .., 24\}$. While the DF method is approximate, reference data at half-filling supports that the spin susceptibility from the dual fermion method is virtually exact at this temperature.[3] In comparison to our AMI result, the spin susceptibility for our perturbative calculation, truncated at fourth order, agrees perfectly with the non-perturbative DF result. Since we compute $\chi_{\uparrow\uparrow}$ and $\chi_{\uparrow\downarrow}$ this implies that the AMI result for $\chi_d$ is equally correct. We see that the DF method underestimates the value of $\chi_d$ in comparison to our main result. This is due to a known bias in the self-consistency applied in the ladder dual-fermion method. Despite these small deviations we observe a two peak structure in DF data with the same peak locations from the non-perturbative calculation as those presented in the


* jleblanc@mun.ca

main paper. This shows that the multi-peak structure in the charge susceptibility is robust and not an artifact of our truncated perturbative expansion.

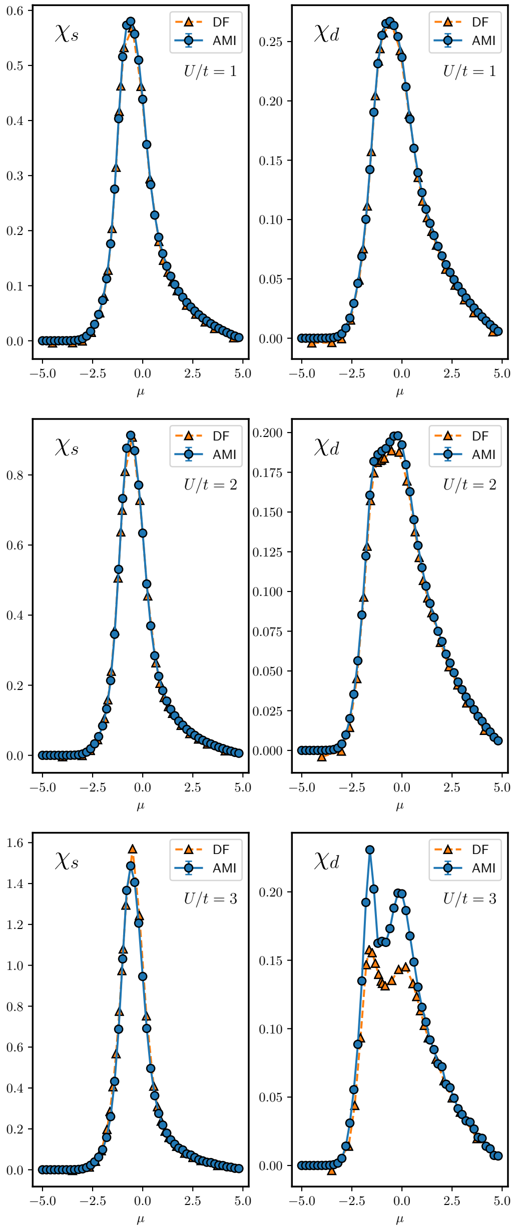


FIG. S2. Spin (left) and charge (right) susceptibilities for $\beta t = 5$, $t'/t = -0.3$ at $U/t = 1$ (top), 2 (middle), 3 (bottom). In addition to AMI data from this work we provide dual Fermion (DF) calculations for comparison.

### B. Compressibility: DMFT

In the main paper we found that for weak-coupling the compressibility, $\kappa = \frac{\partial n}{\partial \mu}$, shows a suppression at a density that does not coincide with half-filling. We perform a similar study using the non-perturbative method of DMFT. Deviations between MBPT and DMFT are expected, since DMFT solves a single site impurity problem self-consistently while MBPT+AMI is in the thermodynamic limit of infinite system size. We present DMFT data in Fig. S3 where we observe a suppression in $\kappa$ similar to that of MBPT+AMI that for $t' \neq 0$ occurs away from half-filling close to the van Hove point of the non-interacting system. Increasing the interaction strength causes the minimum in $\kappa$ to move towards half-filling. We also performed calculations using the non-perturbative dynamical cluster approximation (DCA), an extension of DMFT, for a small 8-site cluster. We see that the compressibility obtained from DCA remains consistent with that of DMFT. Together, these results suggest that the reduction in $\kappa$ away from $n = 0.5$ is a robust feature of the model, captured by both perturbative and non-perturbative methods.

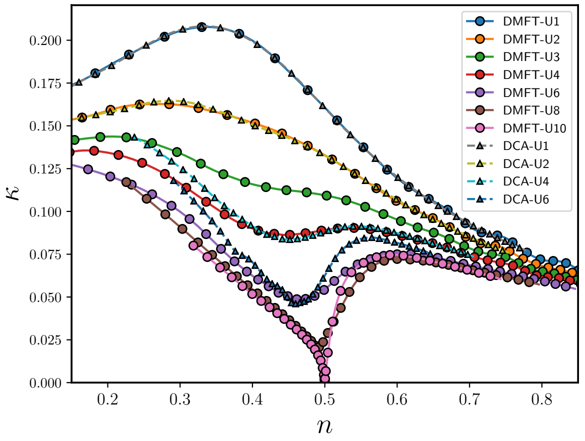


FIG. S3. Results for $\kappa = \frac{\partial n}{\partial \mu}$ at fixed $\beta t = 5$, $t'$ = -0.3 from DMFT and 8-site DCA for variation in $U/t$.

## III. SUPPLEMENTARY NOTE 3: ADDITIONAL DATA

### A. Full $\mu$ Dependence at Low Order

The data presented in the main text Fig. (4) is sparse in choice of densities due to the computational effort required. We present in Fig. S4 lower order calculations, truncated at second order, but for a high resolution grid in chemical potential $\mu$. The splitting in charge and spin excitations noted in the main text at third order exists also at second order. This demonstrates the robust nature of the additional structures in the charge and spin susceptibilities. We see a continual hardening of both spin and charge excitations for increase in chemical potential. We observe nothing particularly special at the half-filled density relative to densities nearby, but do note a maximal splitting in the charge excita-

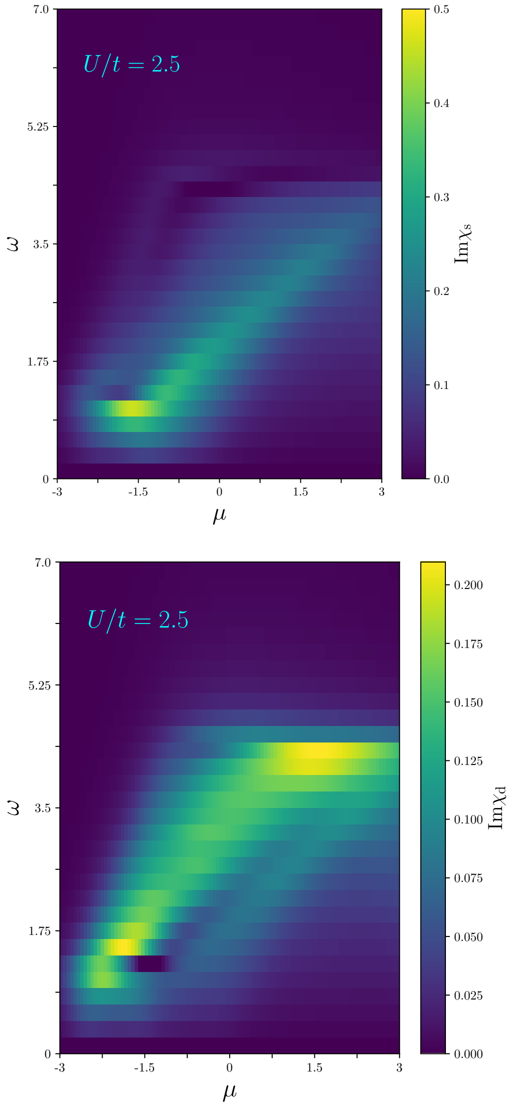


FIG. S4. Imaginary parts of the spin (Top) and charge (Bottom) susceptibilities truncated at second order with $U/t = 2.5$ over a range of $\mu$ and $\omega$ for $\vec{q} = (0, \pi/2)$. A broadening factor of $\Gamma = 0.125$ was used.

tions at chemical potentials near the van Hove point, near $\mu = -1.5 \to -1.2$.

## B. Interaction Strength Dependence

We plot the spin and charge dispersions in Fig. S5 at fixed doping $n = 0.5$ and temperature for momenta along the $\vec{q} = (0, q_y)$ direction for increasing interaction strength. Both spin and charge susceptibilities exhibit clear dispersive behavior with peaks located within a broad incoherent background with the charge excitations showing a linear behavior and occurring at energies

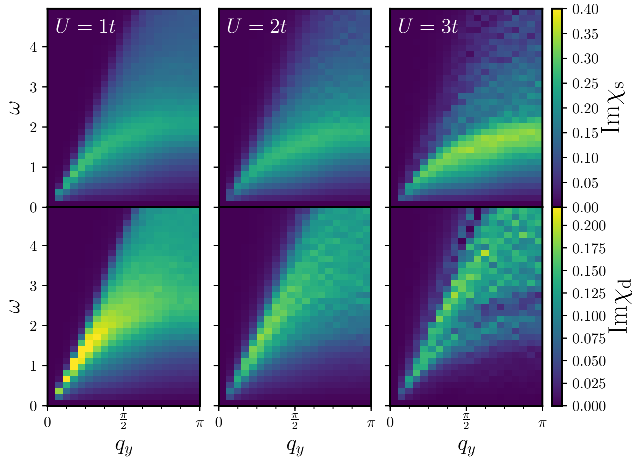


FIG. S5. Imaginary parts of $\chi_s(\omega, q)$ (top) and $\chi_d(\omega, q)$ (bottom) as a function of $\omega$ and $\vec{q} = (0, q_y)$ for $U/t = 1 \to 3$, $t' = -0.3$, and $\beta t = 5$ at a fixed density of $n = 0.5$. Calculations are truncated at third order, as in the main text for real frequency observables. A broadening factor of $\Gamma = 0.125t$ was used.

above the peak in spin excitations. From the progression with interaction strength, we observe a straightforward increase in the spin susceptibility and broadening as $U/t$ increases. In the case of the charge susceptibility, we see at $U/t = 3$ a weak splitting of the charge excitations into a lower and upper peak consistent with Fig. S4 and data presented in the main text.


[1] E. Gull, A. J. Millis, A. I. Lichtenstein, A. N. Rubtsov, M. Troyer, and P. Werner, Rev. Mod. Phys. **83**, 349 (2011).

[2] A. E. Antipov, J. P. F. LeBlanc, and E. Gull, Physics Procedia **68**, 43 (2015), proceedings of the 28th Workshop on Computer Simulation Studies in Condensed Matter Physics (CSP2015).

[3] T. Schäfer, N. Wentzell, F. Šimkovic, Y.-Y. He, C. Hille, M. Klett, C. J. Eckhardt, B. Arzhang, V. Harkov, F. m. c.-M. Le Régent, A. Kirsch, Y. Wang, A. J. Kim, E. Kozik, E. A. Stepanov, A. Kauch, S. Andergassen, P. Hansmann, D. Rohe, Y. M. Vilk, J. P. F. LeBlanc, S. Zhang, A.-M. S. Tremblay, M. Ferrero, O. Parcollet, and A. Georges, Phys. Rev. X **11**, 011058 (2021).
